# Supplementary material for: Low Complexity Deep Learning Augmented Wireless Channel Estimation for Pilot-Based OFDM on Zynq System on Chip
Source: arXiv:2403.01098 source file (2024-03-02)
Supplement: Supplementary file 1 [file 1_appendix.tex]

\appendix

\section{}
The training process in DL is indeed highly dependent on the availability of a sufficient number of training data to effectively train the model.
To address this concern, we conducted experiments where we varied the training dataset size, training the model on smaller datasets. As expected, the BER performance degraded as the training dataset size decreased. In Figure~\ref{fig:datasetSize}, we illustrate the BER performance as a function of the training dataset size.

As observed in the figure, the performance of the LSiDNN is comparable to that of Minimum Mean Square Error (MMSE) at around a dataset size of 5000. However, when further reducing the dataset size to only 5 training samples, the LSiDNN's performance degrades below that of Least Squares (LS). This suggests that the model is not sufficiently trained or maybe overfitted to the limited training data.

    \begin{figure*}[!htbp]
        \centering
        \includegraphics[scale=0.75]{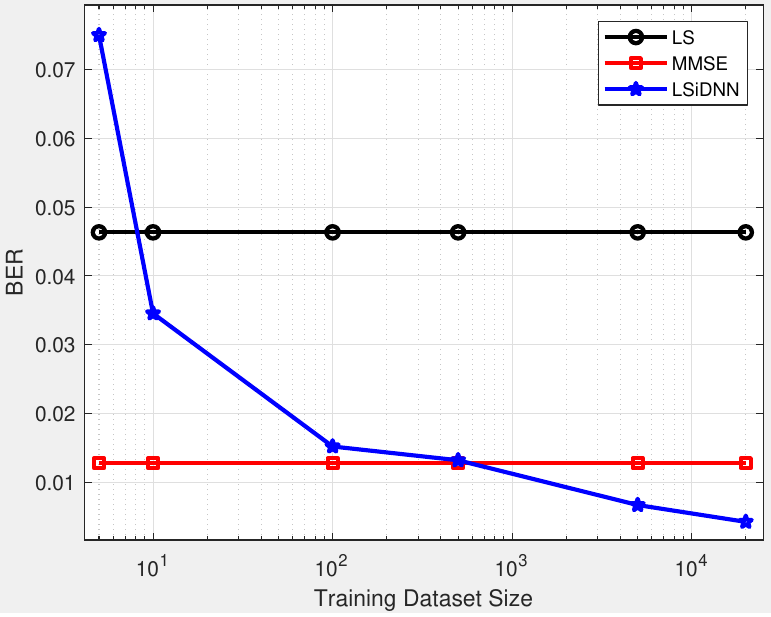}
        \caption{Performance of LSiDNN as a function of dataset Size. }
        \label{fig:datasetSize}
    \end{figure*}
